# Supplementary material for: Probing type-II Ising pairing using the spin-mixing parameter
Source: arXiv:2302.02699 source file (2024-03-26)
Supplement: Supplementary file 1 [file supplementary.tex]

\documentclass[%
aps,amsmath,amssymb, superscriptaddress,
%preprint,%
preprint,%
%author-year,%
%author-numerical,%
]{revtex4-2}

\usepackage[normalem]{ulem}
\usepackage{graphicx}% Include figure files
\usepackage{fancyhdr}
\usepackage[active]{srcltx}
\usepackage{setspace}
\usepackage{float}
\usepackage{bm}% bold math
\usepackage{color}
\usepackage{amsmath}
\usepackage{multirow}

\setcounter{figure}{0}

\usepackage[breaklinks, hidelinks]{hyperref}
\usepackage{xcolor}
\hypersetup{
    colorlinks,
    linkcolor={red!50!black},
    citecolor={red!50!black},
    urlcolor={red!50!black}
}

\begin{document}

\title{Supplemental Material: Probing type-II Ising pairing using the spin-mixing parameter}

\author{Paulina Jureczko}
\affiliation{Institute of Physics, University of Silesia in Katowice, 41-500 Chorzów, Poland}%
\author{Jozef Hani\v{s}}
\affiliation{Institute of Physics, Pavol Jozef \v{S}af\'{a}rik University in Ko\v{s}ice, Park Angelinum 9, 04001 Ko\v{s}ice, Slovakia}

\author{Paulo E. Faria~Junior}
\affiliation{Institute for Theoretical Physics, University of Regensburg, 93040 Regensburg, Germany}

\author{Martin Gmitra}
\email{martin.gmitra@upjs.sk}
\affiliation{Institute of Physics, Pavol Jozef \v{S}af\'{a}rik University in Ko\v{s}ice, Park Angelinum 9, 04001 Ko\v{s}ice, Slovakia}
\affiliation{Institute of Experimental Physics, Slovak Academy of Sciences, Watsonova 47, 04001 Ko\v{s}ice, Slovakia}

\author{Marcin Kurpas}
\email{marcin.kurpas@us.edu.pl}
\affiliation{Institute of Physics, University of Silesia in Katowice, 41-500 Chorzów, Poland}%

\maketitle

\section{Non-relativistic band structures}

\begin{figure}[H]
    \centering
    \includegraphics[width=0.99\textwidth]{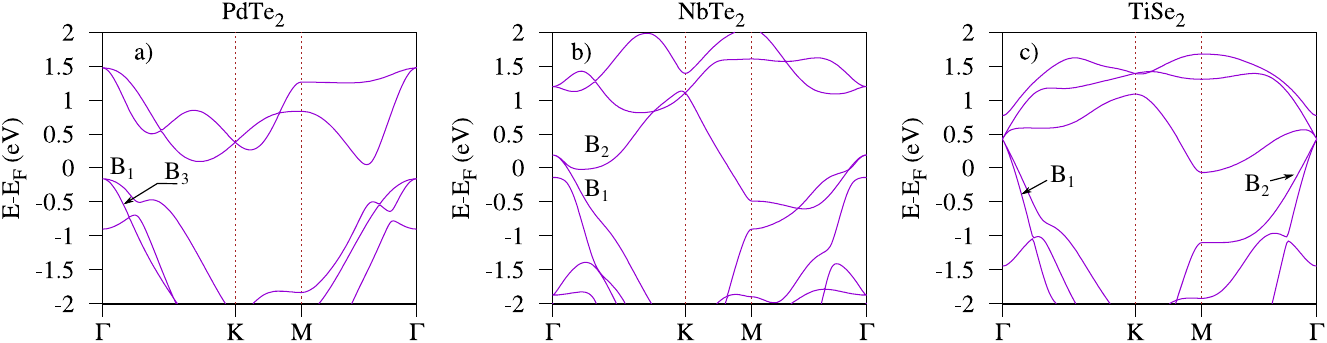}
    \caption{Non-relativistic band structures of (a) PdTe$_2$, (b) TiSe$_2$ and (c) NbTe$_2$ from first principles.}
    \label{fig:S1}
\end{figure}

\begin{figure}[H]
    \centering
    \includegraphics[width=0.7\textwidth]{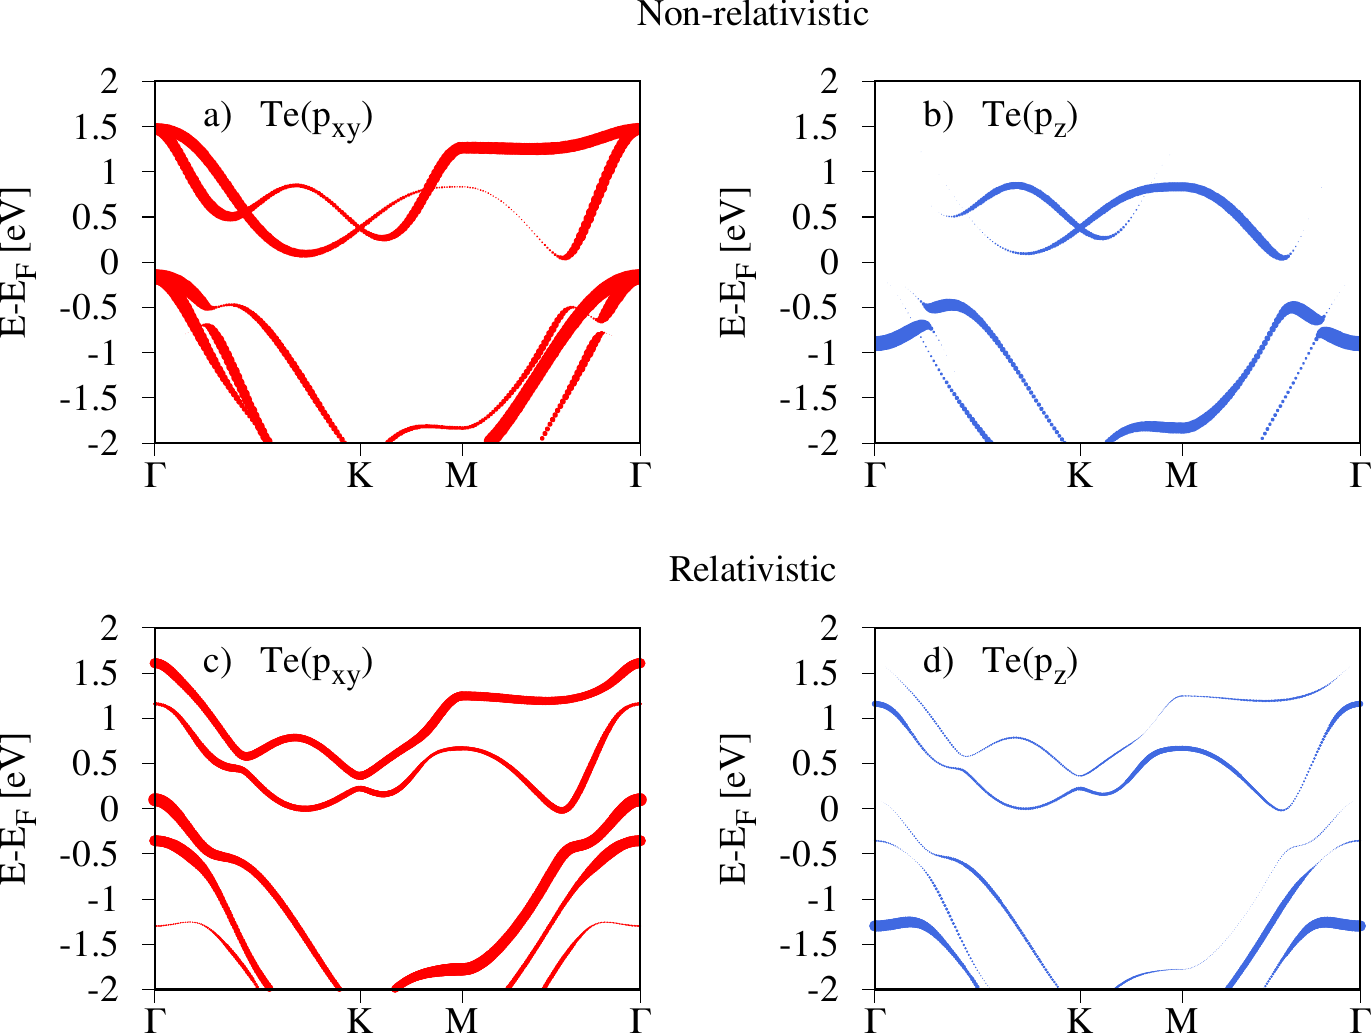}
    \caption{Non-relativistic (a), (b) and relativistic (c), (d) band structure of PdTe$_2$ projected on the atomic Te orbitals.} 
    \label{fig:S2}
\end{figure}

\begin{figure}[H]
    \centering
    \includegraphics[width=0.65\textwidth]{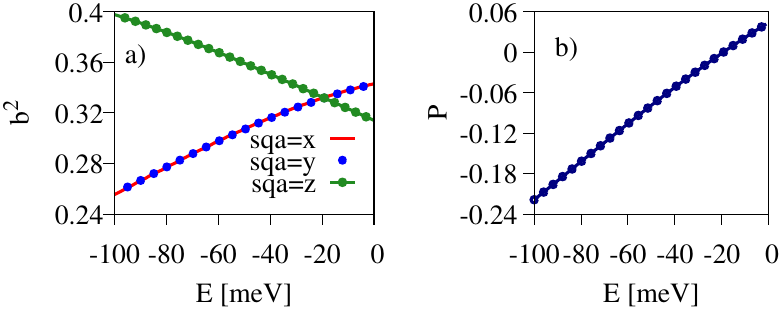}
    \caption{The average value of (a)~the spin-mixing parameter $b^2$ and (b) polarization $P$ in the band $B_3$ of PdTe$_2$, see Fig.~S1 (a), in  the energy range 100\,meV from the top of the band ($E=0$~eV).}
    \label{fig:b2_P_B3_SM}
\end{figure}

\begin{figure}[H] 
    \centering
\includegraphics[width=0.92\textwidth]{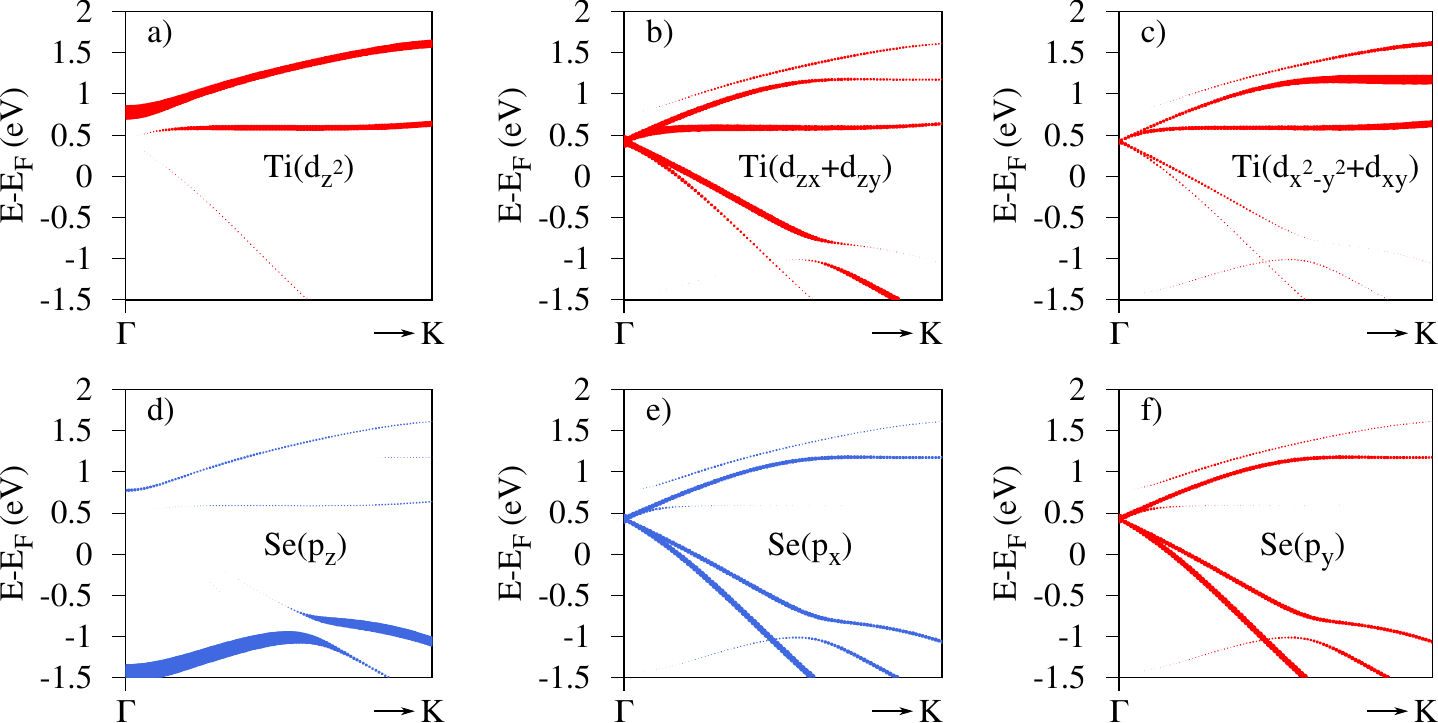}
    \caption{Non-relativistic band structure of TiSe$_2$ close to the $\Gamma$ point projected on the atomic Ti $d$-orbitals and Se $p$-orbitals.}
    \label{fig:S_Tise2_fb_nrel_gamma}
\end{figure}

\section{Symmetry analysis of $\Gamma$-point bands} 

The summary of the relevant irreducible representations (irreps) for the energy bands the $\Gamma$-point are given in Fig.~\ref{fig:irreps}. Our goal is to perform a symmetry analysis of spin-orbit coupling (SOC) terms to rationalize the calculated $b^2$ of the relevant bands B1, B2, and B3 (indicated in Fig.~1(b,g,l) in the main text), following the Refs.~\cite{Kurpas2019, FariaJunior2022NJP}.

\begin{figure*}[htp]
    \centering
    \includegraphics[width=0.99\textwidth]{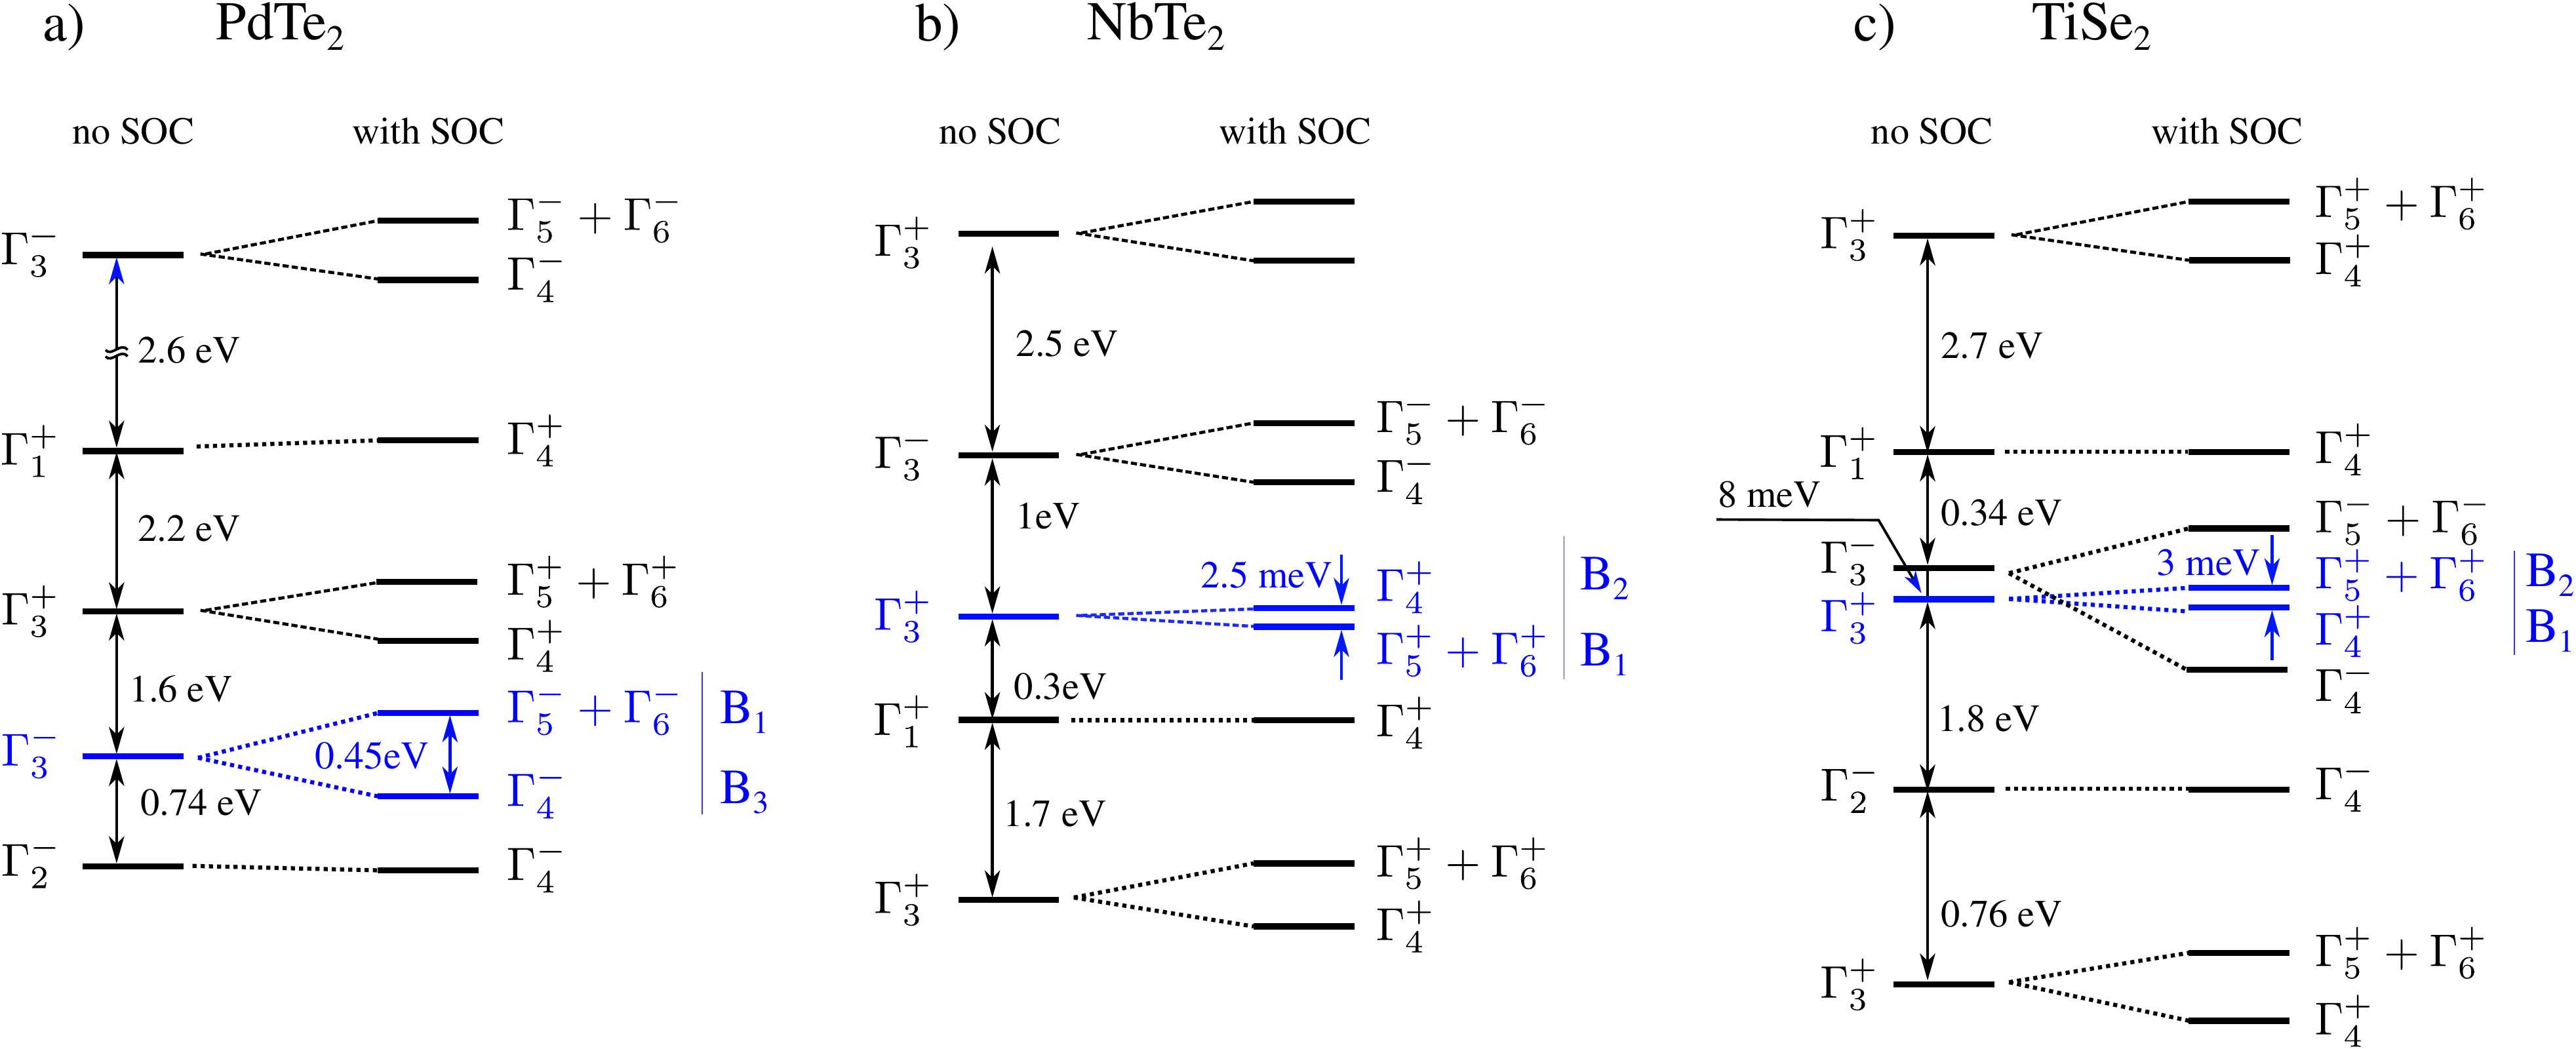}
    \caption{Irreducible representations (irreps) for $\Gamma$-point bands without and with SOC. The irreps in blue indicate the bands B1, B2, and B3 presented in Fig.~1(b,g,l) in the main text.}
    \label{fig:irreps}
\end{figure*}

\begin{table}[h]
\caption{Character table for the group $D_{3d}$.}
\begin{center}
\begin{tabular}{cc|ccc|ccc|cc}
\hline 
\noalign{\vskip0.001\textheight}
$D_{3d}$ &  & $e$ & $2C_{3}$ & \multicolumn{1}{c}{$3C_{2}^{\prime}$} & $i$ & $2S_{6}$ & $3\sigma_{d}$ & \multicolumn{2}{c}{}\tabularnewline[0.001\textheight]
\hline 
\noalign{\vskip0.001\textheight}
$\Gamma_{1}^{+}$ & $A_{1g}$ & 1 & 1 & 1 & 1 & 1 & 1 &  & $x^{2}+y^{2},z^{2}$\tabularnewline[0.001\textheight]
\noalign{\vskip0.001\textheight}
$\Gamma_{2}^{+}$ & $A_{2g}$ & 1 & 1 & -1 & 1 & 1 & -1 & $R_{z}$ & \tabularnewline[0.001\textheight]
\noalign{\vskip0.001\textheight}
$\Gamma_{3}^{+}$ & $E_{g}$ & 2 & -1 & 0 & 2 & -1 & 0 & $\left(R_{x},R_{y}\right)$ & $\left(x^{2}-y^{2},xy\right)$,$\left(xz,yz\right)$\tabularnewline[0.001\textheight]
\cline{3-8} \cline{4-8} \cline{5-8} \cline{6-8} \cline{7-8} \cline{8-8} 
\noalign{\vskip0.001\textheight}
$\Gamma_{1}^{-}$ & $A_{1u}$ & 1 & 1 & 1 & -1 & -1 & -1 &  & \tabularnewline[0.001\textheight]
\noalign{\vskip0.001\textheight}
$\Gamma_{2}^{-}$ & $A_{2u}$ & 1 & 1 & -1 & -1 & -1 & 1 & $z$ & \tabularnewline[0.001\textheight]
\noalign{\vskip0.001\textheight}
$\Gamma_{3}^{-}$ & $E_{u}$ & 2 & -1 & 0 & -2 & 1 & 0 & $\left(x,y\right)$ & \tabularnewline[0.001\textheight]
\hline 
\end{tabular}
\end{center}
\label{tab:D3d}
\end{table}

All the analyzed materials PdTe$_2$, NbTe$_2$, and TiSe$_2$, have a hexagonal lattice with $D_{3d}$ point-group. The character table of the symmetry group $D_{3d}$ is given in Table~\ref{tab:D3d}. The nonzero matrix elements for pseudo-vector operators ($R_x,R_y,R_z$) can be written as
\begin{eqnarray}
\left\langle \Gamma_{1}^{+}\left|R_{x,y} \right|\Gamma_{3}^{+}\right\rangle  & : & \left\langle \Gamma_{1}^{+}\left|R_{x}\right|\Gamma_{3,1}^{+}\right\rangle =\left\langle \Gamma_{1}^{+}\left|R_{y}\right|\Gamma_{3,2}^{+}\right\rangle \nonumber \\
\left\langle \Gamma_{2}^{+}\left|R_{x,y} \right|\Gamma_{3}^{+}\right\rangle  & : & \left\langle \Gamma_{2}^{+}\left|R_{x}\right|\Gamma_{3,2}^{+}\right\rangle =-\left\langle \Gamma_{2}^{+}\left|R_{y}\right|\Gamma_{3,1}^{+}\right\rangle \nonumber \\
\left\langle \Gamma_{3}^{+}\left|R_{x,y} \right|\Gamma_{3}^{+}\right\rangle  & : & \left\langle \Gamma_{3,1}^{+}\left|R_{x}\right|\Gamma_{3,1}^{+}\right\rangle =-\left\langle \Gamma_{3,2}^{+}\left|R_{x}\right|\Gamma_{3,2}^{+}\right\rangle =-\left\langle \Gamma_{3,1}^{+}\left|R_{y}\right|\Gamma_{3,2}^{+}\right\rangle =-\left\langle \Gamma_{3,2}^{+}\left|R_{y}\right|\Gamma_{3,1}^{+}\right\rangle \nonumber \\
\left\langle \Gamma_{1}^{+}\left|R_{z}\right|\Gamma_{2}^{+}\right\rangle  & : & \left\langle \Gamma_{1}^{+}\left|R_{z}\right|\Gamma_{2}^{+}\right\rangle \nonumber \\
\left\langle \Gamma_{3}^{+}\left|R_{z}\right|\Gamma_{3}^{+}\right\rangle  & : & \left\langle \Gamma_{3,1}^{+}\left|R_{z}\right|\Gamma_{3,2}^{+}\right\rangle =-\left\langle \Gamma_{3,2}^{+}\left|R_{z}\right|\Gamma_{3,1}^{+}\right\rangle \label{eq:evenR}
\end{eqnarray}
\begin{eqnarray}
\left\langle \Gamma_{1}^{-}\left|R_{x,y} \right|\Gamma_{3}^{-}\right\rangle  & : & \left\langle \Gamma_{1}^{-}\left|R_{x}\right|\Gamma_{3,1}^{-}\right\rangle =\left\langle \Gamma_{1}^{-}\left|R_{y}\right|\Gamma_{3,2}^{-}\right\rangle \nonumber \\
\left\langle \Gamma_{2}^{-}\left|R_{x,y} \right|\Gamma_{3}^{-}\right\rangle  & : & \left\langle \Gamma_{2}^{-}\left|R_{x}\right|\Gamma_{3,2}^{-}\right\rangle =-\left\langle \Gamma_{2}^{-}\left|R_{y}\right|\Gamma_{3,1}^{-}\right\rangle \nonumber \\
\left\langle \Gamma_{3}^{-}\left|R_{x,y} \right|\Gamma_{3}^{-}\right\rangle  & : & \left\langle \Gamma_{3,1}^{-}\left|R_{x}\right|\Gamma_{3,1}^{-}\right\rangle =-\left\langle \Gamma_{3,2}^{-}\left|R_{x}\right|\Gamma_{3,2}^{-}\right\rangle =-\left\langle \Gamma_{3,1}^{-}\left|R_{y}\right|\Gamma_{3,2}^{-}\right\rangle =-\left\langle \Gamma_{3,2}^{-}\left|R_{y}\right|\Gamma_{3,1}^{-}\right\rangle \nonumber \\
\left\langle \Gamma_{1}^{-}\left|R_{z}\right|\Gamma_{2}^{-}\right\rangle  & : & \left\langle \Gamma_{1}^{-}\left|R_{z}\right|\Gamma_{2}^{-}\right\rangle \nonumber \\
\left\langle \Gamma_{3}^{-}\left|R_{z}\right|\Gamma_{3}^{-}\right\rangle  & : & \left\langle \Gamma_{3,1}^{-}\left|R_{z}\right|\Gamma_{3,2}^{-}\right\rangle =-\left\langle \Gamma_{3,2}^{-}\left|R_{z}\right|\Gamma_{3,1}^{-}\right\rangle \label{eq:oddR}
\end{eqnarray}
and, essentially, the same relations connecting the non-zero matrix elements apply for even or odd irreps. Pseudo-vector operators only connect irreps with the same parity.

The SOC term is written as
\begin{eqnarray}
\mathbf{H}_{\rm SO} & = & \frac{\hbar}{4m_{0}^{2}c^{2}}\left(\vec{\nabla}V\times\vec{p}\right)\cdot\vec{\sigma} \nonumber  \\  
 & = & \underset{H_{{\rm SO}x}\sim R_{x}}{\underbrace{\left[\frac{\hbar}{4m_{0}^{2}c^{2}}\left(\frac{\partial V}{\partial y}p_{z}-\frac{\partial V}{\partial z}p_{y}\right)\right]}}\sigma_{x}
 +\underset{H_{{\rm SO}y}\sim R_{y}}{\underbrace{\left[\frac{\hbar}{4m_{0}^{2}c^{2}}\left(\frac{\partial V}{\partial z}p_{x}-\frac{\partial V}{\partial x}p_{z}\right)\right]}}\sigma_{y} \nonumber \\
 & & +\underset{H_{{\rm SO}z}\sim R_{z}}{\underbrace{\left[\frac{\hbar}{4m_{0}^{2}c^{2}}\left(\frac{\partial V}{\partial x}p_{y}-\frac{\partial V}{\partial y}p_{x}\right)\right]}}\sigma_{z}
\end{eqnarray}

The relevant bands of interest, indicated in blue color in Fig.~\ref{fig:irreps}, below to $\Gamma^-_3$ or $\Gamma^+_3$ without SOC. Let us focus on the irrep $\Gamma^-_3$ to investigate the role of intraband and interband SOC. 
The intraband SOC Hamiltonian for the states $\left\{ \left|\Gamma_{3,1}^{-}\uparrow\right\rangle ,\left|\Gamma_{3,2}^{-}\uparrow\right\rangle ,\left|\Gamma_{3,1}^{-}\downarrow\right\rangle ,\left|\Gamma_{3,2}^{-}\downarrow\right\rangle \right\}$ only present a contribution from the $H_{{\rm SO}z}$ term since the $H_{{\rm SO}x,y}$ terms are forbidden by time-reversal symmetry. The Hamiltonian reads
\begin{equation}
\left[\begin{array}{cccc}
0 & i\Delta_{z} & 0 & 0\\
-i\Delta_{z} & 0 & 0 & 0\\
0 & 0 & 0 & -i\Delta_{z}\\
0 & 0 & i\Delta_{z} & 0
\end{array}\right]
\end{equation}
\\
with $\left\langle \Gamma_{3,1}^{-}\left|H_{{\rm SO}z}\right|\Gamma_{3,2}^{-}\right\rangle =-\left\langle \Gamma_{3,2}^{-}\left|H_{{\rm SO}z}\right|\Gamma_{3,1}^{-}\right\rangle =i\Delta_{z}$.

The solutions for this Hamiltonian are given by:
\begin{align}
\Delta_{z} & \rightarrow\left|\Gamma_{3-}^{-}\uparrow\right\rangle ,\left|\Gamma_{3+}^{-}\downarrow\right\rangle \nonumber \\
-\Delta_{z} & \rightarrow\left|\Gamma_{3+}^{-}\uparrow\right\rangle ,\left|\Gamma_{3-}^{-}\downarrow\right\rangle 
\end{align}
with
\begin{align}
\left|\Gamma_{3\pm}^{-}\uparrow\right\rangle  & =\frac{1}{\sqrt{2}}\left(\left|\Gamma_{3,1}^{-}\right\rangle \pm i\left|\Gamma_{3,2}^{-}\right\rangle \right)\left|\uparrow\right\rangle \nonumber \\
\left|\Gamma_{3\pm}^{-}\downarrow\right\rangle  & =\frac{1}{\sqrt{2}}\left(\left|\Gamma_{3,1}^{-}\right\rangle \pm i\left|\Gamma_{3,2}^{-}\right\rangle \right)\left|\downarrow\right\rangle 
\end{align}
The intraband SOC term $\Delta_z$ is capable of splitting the energy of opposite spins but does not introduce any spin-mixing. Such spin-mixing arises from the interband SOC. In order to identify the relevant bands that contribute to the spin-mixing and rationalize the magnitude of $b^{2}$ at the $\Gamma$-point, we evaluate the non-zero corrections to the wave function within 1st order perturbation theory with respect to the
$\mathbf{H}_{\rm SO}$ term, i. e.,
\begin{equation}
\left|\Gamma_{3\alpha}^{-}\tilde{\sigma}\right\rangle =\left|\Gamma_{3\alpha}^{-}\sigma\right\rangle +\underset{b}{\overset{B}{\sum}}\frac{\left\langle b\left|\mathbf{H}_{\rm SO}\right|\Gamma_{3\alpha}^{-}\sigma\right\rangle }{E(\Gamma_{3\alpha}^{-}\sigma)-E(b)}\left|b\right\rangle 
\end{equation}
\\
with $\alpha=\pm$, $\sigma=\uparrow,\downarrow$~... The $\sim$ indicates the renormalized spin values $\tilde{\sigma}=\Uparrow,\Downarrow$ after the mixing. The subset $B$ comprises all the other odd irreps present in the system, i.e., $B=\left\{ \Gamma_{1}^{-}\oplus\Gamma_{2}^{-}\oplus\Gamma_{3}^{-}\right\} \otimes\left\{ \uparrow,\downarrow\right\}$ (the even irreps are not included since they do not contribute to the coupling, see Eq.~(\ref{eq:oddR})). The symmetry analysis allows us to write:
\begin{align}
\left|\Gamma_{3-}^{-}\Uparrow\right\rangle  & =\left|\Gamma_{3-}^{-}\uparrow\right\rangle +\underset{\beta}{\overset{\Gamma_{3}^{-}}{\sum}}\frac{\left\langle \beta\left|H_{{\rm SO}z}\sigma_{z}\right|\Gamma_{3-}^{-}\uparrow\right\rangle }{E(\Gamma_{3-}^{-}\uparrow)-E(\beta)}\left|\beta\uparrow\right\rangle \nonumber \\
 & +\underset{\beta}{\overset{\Gamma_{1}^{-},\Gamma_{2}^{-}}{\sum}}\frac{\left\langle \beta\downarrow\left|H_{{\rm SO}x}\sigma_{x}+H_{{\rm SO}y}\sigma_{y}\right|\Gamma_{3-}^{-}\uparrow\right\rangle }{E(\Gamma_{3-}^{-}\uparrow)-E(\beta)}\left|\beta\downarrow\right\rangle 
\end{align}
\begin{align}
\left|\Gamma_{3+}^{-}\Downarrow\right\rangle  & =\left|\Gamma_{3+}^{-}\downarrow\right\rangle +\underset{\beta}{\overset{\Gamma_{3}^{-}}{\sum}}\frac{\left\langle \beta\left|H_{{\rm SO}z}\sigma_{z}\right|\Gamma_{3-}^{-}\downarrow\right\rangle }{E(\Gamma_{3-}^{-}\downarrow)-E(\beta)}\left|\beta\downarrow\right\rangle \nonumber \\
 & +\underset{\beta}{\overset{\Gamma_{1}^{-},\Gamma_{2}^{-}}{\sum}}\frac{\left\langle \beta\uparrow\left|H_{{\rm SO}x}\sigma_{x}+H_{{\rm SO}y}\sigma_{y}\right|\Gamma_{3+}^{-}\downarrow\right\rangle }{E(\Gamma_{3+}^{-}\downarrow)-E(\beta)}\left|\beta\uparrow\right\rangle 
\end{align}
\begin{align}
\left|\Gamma_{3+}^{-}\Uparrow\right\rangle  & =\left|\Gamma_{3+}^{-}\uparrow\right\rangle +\underset{\beta}{\overset{\Gamma_{3}^{-}}{\sum}}\frac{\left\langle \beta\left|H_{{\rm SO}z}\sigma_{z}\right|\Gamma_{3+}^{-}\uparrow\right\rangle }{E(\Gamma_{3+}^{-}\uparrow)-E(\beta)}\left|\beta\uparrow\right\rangle \nonumber \\
 & +\underset{\beta}{\overset{\Gamma_{3}^{-}}{\sum}}\frac{\left\langle \beta\downarrow\left|H_{{\rm SO}x}\sigma_{x}+H_{{\rm SO}y}\sigma_{y}\right|\Gamma_{3+}^{-}\uparrow\right\rangle }{E(\Gamma_{3+}^{-}\uparrow)-E(\beta)}\left|\beta\downarrow\right\rangle 
\end{align}
\begin{align}
\left|\Gamma_{3-}^{-}\Downarrow\right\rangle  & =\left|\Gamma_{3-}^{-}\downarrow\right\rangle +\underset{\beta}{\overset{\Gamma_{3}^{-}}{\sum}}\frac{\left\langle \beta\left|H_{{\rm SO}z}\sigma_{z}\right|\Gamma_{3-}^{-}\downarrow\right\rangle }{E(\Gamma_{3-}^{-}\downarrow)-E(\beta)}\left|\beta\downarrow\right\rangle \nonumber \\
 & +\underset{\beta}{\overset{\Gamma_{3}^{-}}{\sum}}\frac{\left\langle \beta\uparrow\left|H_{{\rm SO}x}\sigma_{x}+H_{{\rm SO}y}\sigma_{y}\right|\Gamma_{3-}^{-}\downarrow\right\rangle }{E(\Gamma_{3-}^{-}\downarrow)-E(\beta)}\left|\beta\uparrow\right\rangle 
\end{align}

And therefore, in summary, we found that:
\begin{align}
\Delta_{z} & \rightarrow\left|\Gamma_{3-}^{-}\Uparrow\right\rangle ,\left|\Gamma_{3+}^{-}\Downarrow\right\rangle \rightarrow\text{spin-mixed with }\Gamma_{1}^{-},\Gamma_{2}^{-}\text{ bands}\nonumber \\
-\Delta_{z} & \rightarrow\left|\Gamma_{3+}^{-}\Uparrow\right\rangle ,\left|\Gamma_{3-}^{-}\Downarrow\right\rangle \rightarrow\text{spin-mixed with }\Gamma_{3}^{-}\text{ bands}
\end{align}
which is also valid for $\Gamma_3^+$ bands, which we write down for completeness
\begin{align}
\Delta_{z} & \rightarrow\left|\Gamma_{3-}^{+}\Uparrow\right\rangle ,\left|\Gamma_{3+}^{+}\Downarrow\right\rangle \rightarrow\text{spin-mixed with }\Gamma_{1}^{+},\Gamma_{2}^{+}\text{ bands}\nonumber \\
-\Delta_{z} & \rightarrow\left|\Gamma_{3+}^{+}\Uparrow\right\rangle ,\left|\Gamma_{3-}^{+}\Downarrow\right\rangle \rightarrow\text{spin-mixed with }\Gamma_{3}^{+}\text{ bands}
\end{align}

By inspecting the neighboring bands in Fig.~\ref{fig:irreps}, we can make the following statements about $b^2$ (assuming spin-quantization axis along the $z$-direction):
\begin{itemize}
   \item PdTe$_2$: there is a $\Gamma^-_2$ band 0.74 eV below the relevant $\Gamma^-_3$ band and a second $\Gamma^-_3$ band 6.4 eV above the relevant $\Gamma^-_3$ band. Therefore, $b^2$ should be much smaller for $\left|\Gamma_{3+}^{-}\Uparrow\right\rangle ,\left|\Gamma_{3-}^{-}\Downarrow\right\rangle$ than for $\left|\Gamma_{3-}^{-}\Uparrow\right\rangle ,\left|\Gamma_{3+}^{-}\Downarrow\right\rangle$.

   \item NbTe$_2$: there is a $\Gamma^+_1$ band 0.3 eV below the relevant $\Gamma^+_3$ band and two $\Gamma^+_3$ bands 3.5 eV above and 2 eV below the relevant $\Gamma^+_3$ band. Therefore, $b^2$ should be smaller for $\left|\Gamma_{3+}^{+}\Uparrow\right\rangle ,\left|\Gamma_{3-}^{+}\Downarrow\right\rangle$ than for $\left|\Gamma_{3-}^{+}\Uparrow\right\rangle ,\left|\Gamma_{3+}^{+}\Downarrow\right\rangle$. 

   \item TiSe$_2$: there is a $\Gamma^+_1$ band 0.348 eV above the relevant $\Gamma^+_3$ band and two $\Gamma^+_3$ bands 3.048 eV above and 2.56 eV below the relevant $\Gamma^+_3$ band. Therefore, $b^2$ should be smaller for $\left|\Gamma_{3+}^{+}\Uparrow\right\rangle ,\left|\Gamma_{3-}^{+}\Downarrow\right\rangle$ then for $\left|\Gamma_{3-}^{+}\Uparrow\right\rangle ,\left|\Gamma_{3+}^{+}\Downarrow\right\rangle$.
\end{itemize}

This would allow us to identify the double group irreps $\Gamma^\pm_4$ and $\Gamma^\pm_5\oplus\Gamma^\pm_6$ and the sign of the intraband SOC splitting $\Delta_z$, which we summarize in Table~\ref{tab:bandsb2}.

\begin{table}[ht]
\caption{$b_z^2$ calculated for SQA=$z$. DG stands for double group and ADG for adapted double group.}
\begin{center}
\begin{tabular}{cccccccccccccccc}
\hline 
\hline 
\noalign{\vskip0.001\textheight}
 &  & $\quad$ &  & $\quad$ &  & Band & $\quad$ &  & $b_z^{2}$ & $\quad$ &  & DG irrep & $\quad$ &  & ADG irrep\tabularnewline[0.001\textheight]
\hline 
\noalign{\vskip0.001\textheight}
\multirow{2}{*}{PdTe$_{2}$} & \multirow{2}{*}{} & \multirow{2}{*}{} & \multirow{2}{*}{$\Delta_{z}<0$} &  &  & B1 &  &  & 0.000000488 &  &  & $\Gamma_{5}^{-}\oplus\Gamma_{6}^{-}$ &  &  & $\left|\Gamma_{3+}^{-}\Uparrow\right\rangle ,\left|\Gamma_{3-}^{-}\Downarrow\right\rangle $\tabularnewline[0.001\textheight]
\noalign{\vskip0.001\textheight}
 &  &  &  &  &  & B3 &  &  & 0.314013252 &  &  & $\Gamma_{4}^{-}$ &  &  & $\left|\Gamma_{3-}^{-}\Uparrow\right\rangle ,\left|\Gamma_{3+}^{-}\Downarrow\right\rangle $\tabularnewline[0.001\textheight]
\hline 
\noalign{\vskip0.001\textheight}
\multirow{2}{*}{NbTe$_{2}$} & \multirow{2}{*}{} & \multirow{2}{*}{} & \multirow{2}{*}{$\Delta_{z}>0$} &  &  & B1 &  &  & 0.000672534 &  &  & $\Gamma_{5}^{+}\oplus\Gamma_{6}^{+}$ &  &  & $\left|\Gamma_{3+}^{+}\Uparrow\right\rangle ,\left|\Gamma_{3-}^{+}\Downarrow\right\rangle $\tabularnewline[0.001\textheight]
\noalign{\vskip0.001\textheight}
 &  &  &  &  &  & B2 &  &  & 0.051897678 &  &  & $\Gamma_{4}^{+}$ &  &  & $\left|\Gamma_{3-}^{+}\Uparrow\right\rangle ,\left|\Gamma_{3+}^{+}\Downarrow\right\rangle $\tabularnewline[0.001\textheight]
\hline 
\noalign{\vskip0.001\textheight}
\multirow{2}{*}{TiSe$_{2}$} & \multirow{2}{*}{} & \multirow{2}{*}{} & \multirow{2}{*}{$\Delta_{z}<0$} &  &  & B1 &  &  & 0.004137026 &  &  & $\Gamma_{4}^{+}$ &  &  & $\left|\Gamma_{3-}^{+}\Uparrow\right\rangle ,\left|\Gamma_{3+}^{+}\Downarrow\right\rangle $\tabularnewline[0.001\textheight]
\noalign{\vskip0.001\textheight}
 &  &  &  &  &  & B2 &  &  & 0.000038732 &  &  & $\Gamma_{5}^{+}\oplus\Gamma_{6}^{+}$ &  &  & $\left|\Gamma_{3+}^{+}\Uparrow\right\rangle ,\left|\Gamma_{3-}^{+}\Downarrow\right\rangle $\tabularnewline[0.001\textheight]
\hline
\hline 
\end{tabular}
\end{center}
\label{tab:bandsb2}
\end{table}

%--------------------------------------
%--------------------------------------
\section{Estimation of $B_{c2,\parallel}$} 

We estimate the temperature dependence of the in-plane upper critical magnetic field $B_{\textrm{c2},\parallel}$ using the microscopic model for single band superconductivity developed in Ref. \cite{LiuPRX_2018}:

\begin{equation}\label{eq:Bc2}
\ln\left(\frac{T}{T_{c}}\right) + \frac{\mu_{B}^{2}B_{c2,\parallel}}{\widetilde{\beta_{\rm SO}^{2}} + \mu_{B}^{2}B_{c2,\parallel}}\,Re \left[ \psi \left( \frac{1}{2} + \frac{i\sqrt{\widetilde{\beta_{\rm SO}^{2}} + \mu_{B}^{2}B_{c2,\parallel}}}{2\pi k_{B}T}\right) - \psi \left(\frac{1}{2}\right)                   \right] = 0,
\end{equation}
where $\widetilde{\beta_{\rm SO}} = B_{\perp}/\left(1+\frac{\hbar}{2 \pi k_{\rm B}T_{c}\tau_{0}}\right)$ is the effective Zeeman SOC strength due to the out-of-plane component of the intrinsic SOC field $B_{\perp}$, $T_c$ is the critical temperature, $\mu_{\textrm{B}}$ is the Bohr magneton, $\tau_0$ is momentum lifetime, and $\psi(x)$ is the digamma function. The  model was used to extract $B_{\textrm{c2},\parallel}$ for PdTe$_2$ from experimental data in Ref. \cite{Liu2020}. To  provide realistic estimations on $B_{\textrm{c2},\parallel}$, we use the values of $T_c = 0.7$\,K and $\tau_0 = 7.25$\,fs extracted from  Ref. \cite{Liu2020}.

\begin{figure}[H]
    \centering
\includegraphics[width=0.7\columnwidth]{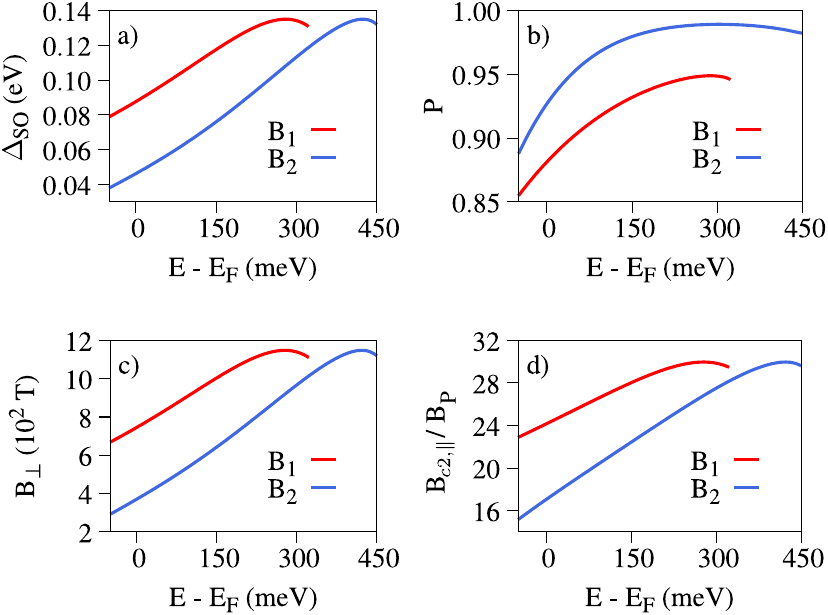}
    \caption{Calculated average (a) spin-orbital gap $\Delta_{\textrm{so}}$, (b) polarization $P$, out-of-plane intrinsic SOC field amplitude and (d) in-plane upper critical field $B_{\textrm{c2},\parallel}$(0\;K) for the $B_1$ and $B_2$ bands of monolayer TiSe$_2$ around the $\Gamma$ point [see Fig. 1 l) in the main text] plotted as a function of the Fermi level varying from $-50$\,meV up to the top of the band at the $\Gamma$ point. Differences in $\Delta_{so}$ and other quantities between the bands $B_1$ and $B_2$ come from different energy dispersion (effective masses) of these bands leading to different Fermi contours at a given Fermi energy. }
    \label{fig:S_tise2_4plot}
\end{figure}

\begin{figure}[H] 
    \centering
\includegraphics[width=0.65\textwidth]{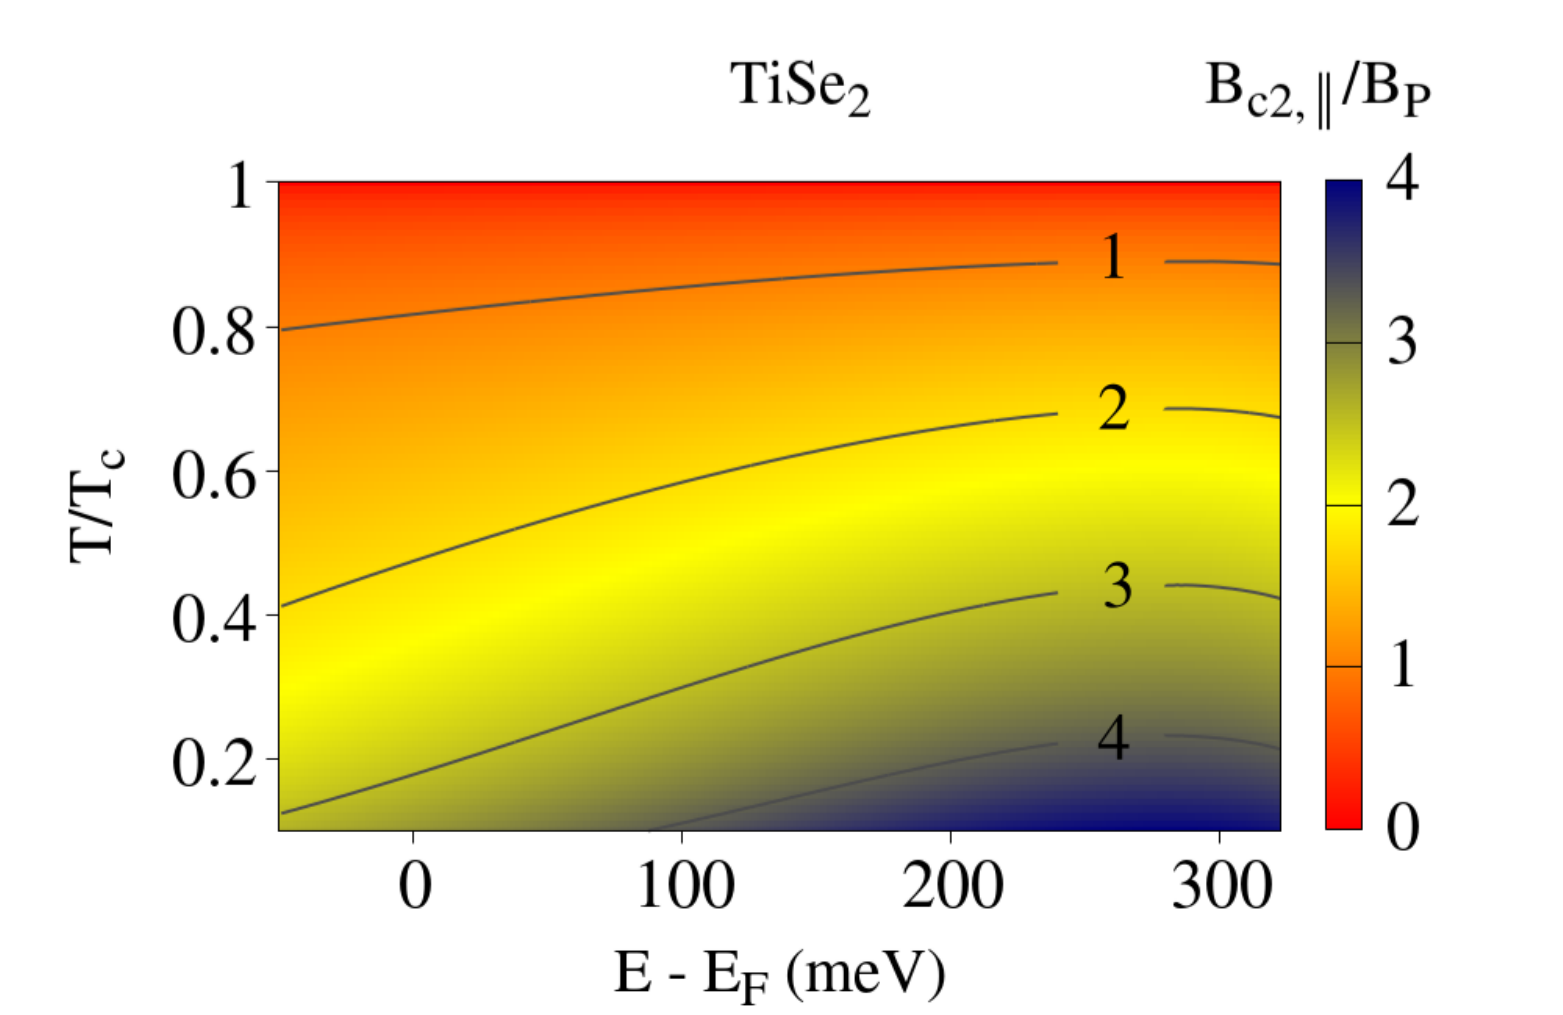}
    \caption{The upper critical field $B_{c2,||}$  versus temperature and the Fermi level for the band B$_1$ of  TiSe$_2$ [see Fig. 1 l) in the main text] estimated using Eq. (\ref{eq:Bc2}).}
    \label{fig:is_model_cont_B1.png}
\end{figure}

\bibliography{bibliography}

\end{document}
